# Supplementary material for: Probe before You Talk: Towards Black-box Defense against Backdoor Unalignment for Large Language Models
Source: arXiv:2506.16447 source file (2025-06-19)
Supplement: Supplementary file 1 [file appendix.tex]

% \paragraph{Defenses.}
% We compare NAS with existing gray-box/black-box backdoor sample detection methods for NLP models.
% (1) \textbf{STRIP}~\cite{strip2} that perturbs the input repeatedly and uses the mean prediction entropy to obtain the anomaly score. 
% (2) \textbf{ONION}~\cite{onion} purifies backdoor samples by removing words that cause an abnormal increase in perplexity (PPL) based on adding context-independent trigger words compromises textual fluency. Here, we follow~\cite{rap} to adjust it as a detection baseline, employing the maximum PPL increase during the process of discarding words one by one as the anomaly score.  
% (3) \textbf{DAN}~\cite{maha_distance} that calculates the Mahalanobis distance between input and clean validation datasets in output probability distribution of last token as the anomaly score.

\input{Tex/appendix/config}
\input{Tex/appendix/additional_results}
